# Supplementary material for: ConsistRM: Improving Generative Reward Models via Consistency-Aware Self-Training
Source: arXiv:2604.07484 source file (2026-04-20)
Supplement: Supplementary file 1 [file 8_Appendix.tex]

% This file compiles with both LuaLaTeX and XeLaTeX
\documentclass[11pt]{article}

% Change "review" to "final" to generate the final (sometimes called camera-ready) version.
% Change to "preprint" to generate a non-anonymous version with page numbers.
\usepackage[review]{acl}

% This is not strictly necessary, and may be commented out,
% but it will improve the layout of the manuscript,
% and will typically save some space.
\usepackage{microtype}
\usepackage{amsmath}
\usepackage{algorithm}
\usepackage{algorithmic}
\usepackage{algorithmicx}
% \usepackage{algpseudocode}

 % \usepackage{algorithmicx}

% If the title and author information does not fit in the area allocated, uncomment the following
%
%\setlength\titlebox{<dim>}
%
% and set <dim> to something 5cm or larger.

% These font selection commands work with
% LuaLaTeX and XeLaTeX, but not pdfLaTeX.
\usepackage[english,bidi=default]{babel} % English as the main language.
\babelfont{rm}{TeXGyreTermesX} % similar to Times
%%% include whatever languages you need below this line
\babelprovide[import]{hindi}
\babelfont[*devanagari]{rm}{Lohit Devanagari}
\babelprovide[import]{arabic}
\babelfont[*arabic]{rm}{Noto Sans Arabic}

\begin{document}
\section{Appendix}
\subsection{Training Configuration}

\subsection{Prompt for Training}

\subsection{Case Study}

\end{document}
